# Supplementary material for: Stability of Underdominant Genetic Polymorphisms in Population Networks
Source: arXiv:1509.02205 source file (2015-09-27)
Supplement: Supplementary file 1 [file laruson20150908supparxiv.tex]

\documentclass[11pt,a4paper]{article}
\usepackage[utf8]{inputenc}

\usepackage{amssymb}
\usepackage{amsmath}
\usepackage{mathrsfs}
\usepackage{graphicx}
\usepackage{url}
\usepackage{lineno}

\usepackage[round]{natbib}

\bibliographystyle{plainnat}

\begin{document}

\begin{center}
{\Large \textsc{Supplemental Material: Stability of Underdominant Genetic Polymorphisms in Population Networks}}
\\
\textsc{\\ \'Aki J.~L\'aruson and Floyd A.~Reed}
\end{center}

\section{\label{Introduction} Introduction}

Genes are found in different forms, referred to as alleles, in a population.  For most genes in most multicellular species gene copies are paired as a diploid genotype. The average fitness of a genotype can be interpreted as the relative abundance of fertile offspring resulting from individuals that have the corresponding genotype. 

In addition to considering the effects of a single gene, a well understood form of underdominance derives from the physical arrangement of multiple genes along linear chromosomes.  Speaking very generally the large scale arrangement of gene order is consistent within a species; however, types of mutations can occur that result in chromosomal rearrangements.  This leads to an effective reduction in fertility of individuals heterozygous for a chromosomal rearrangements, due to segmental aneuploidy (an extra or missing gene copy that disrupts normal gene expression levels) among the offspring \citep{Snell1946}.

\section{\label{Methods and Results} Methods and Results}

There are a number of reasonable alternative ways to incorporate migration into the network.  Here we are explicitly interested in the effect of the network topology. We decided to have each edge conduct the same fraction of migrants into a node so that nodes with more connections will experience a greater exchange of alleles with neighbouring populations. This seems biologically reasonable and additional elaborations, such as a distribution of longer distance migration (beyond immediately adjacent nodes), which also has strong biological motivation, were not addressed here.

Each generation, $g$, the allele frequency, $p$ of each population node, $i$, is updated with the fraction of immigrants from $n$ adjacent populations, $j$, at a migration rate of $m$.  

$$p_{i,g} = (1 - c_i m) p_{i,g-1} + \sum_{j=1}^N m a_{i,j} p_{j,g-1}$$ 

Note that this equation will not be appropriate if the fraction of alleles introduced into a population exceeded unity. One possible approach is to modify the equation as follows.

$$p_{i,g} = \frac{p_{i,g-1} + \sum_{j=1}^N m a_{i,j} p_{j,g-1}}{1 + c_i m}$$ 

However, this means that the migration rates will not be uniform for each edge and that effective migration rates will be increasingly overestimated as $c_i m$ becomes large. We have not used this modification in the current manuscript but it may prove useful in later applications.

\subsubsection{Random Graphs}

\begin{table}[ht]
\caption{\label{rtab} Pearson's correlation coefficient for selected network summary statistics. Unless indicated otherwise the range of nodes evaluated was a uniform random variable distributed from $2 \le V \le 20$.  The range of edges were a uniform random variable chosen from $V-1 \le E \le V(V-1)/2$, which is the maximum and minimum number of edges possible for a connected network given $V$. A heterozygote fitness of $\omega=1/2$ was used. 
 All correlations were significant at a $P<0.05$}
\begin{tabular}{ | l | c | c | c | c | }
  \hline			
  Pearson's $r$ & Full Range & $V=10$ & $E=10$ & $V=E=10$ \\
  \hline	
  $V$ & -0.2488 & --- & 0.8000 & --- \\
  \hline	
  $E$ & -0.4825 & -0.6917 & --- & --- \\
  \hline  
  $V/E$ & 0.5929 & 0.8430 & 0.8000 & --- \\
  \hline 
  Variance & -0.4882 & -0.6332 & -0.4237 & -0.1239 \\
  \hline 
  Variance$/E$ & 0.0098 & -0.5104 & -0.4237 & -0.1239 \\
  \hline 
  Efficiency & 0.1931 & -0.6896 & -0.7038 & 0.0614 \\
  \hline 
  Diameter & 0.6058 & 0.8401 & 0.7071 & 0.2651 \\
  \hline 
  Dendricity & 0.4828 & 0.5714 & 0.6067 & 0.2342 \\
  \hline 
  Evenness & 0.0959 & --- & 0.1413 & --- \\
  \hline 
  Terminalness & 0.5184 & 0.7891 & 0.7281 & -0.0516 \\
  \hline 
\end{tabular}
\end{table}

\section{\label{Discussion} Discussion}

\subsection{The coordination game}  
 
Many processes, in addition to the classic stag hunt scenario \citep{Skyrms2001}, can be interpreted in terms of the coordination game.  For example, the choice of which language to learn and use to communicate \citep[the language diversity of the Bismark and Solomon archipelagos,][and the treelike network they form with the coastal Papua New Guinea mainland is an interesting example]{Dunn2002}, which side of the road to drive on, the type of common currency to use in economic trade, or simply a time and place to meet regularly (periodic market-day circuits \citep{Eighmy1972,Park1981}, with a preponderance of even-day routes \citep{Hill1966}, versus ``dendritic'' trade-distribution routes and the maintanence of non-uniform pricing \citep{Smith1974} are also interesting examples in the present context), are all processes that typically have a higher payoff when the same strategy, out of a range of possibly equivalent strategies, is adopted. This is related to the idea of standardization in economics and these dynamics are associated with multiple Nash equilibria (a single player cannot increase their payoff by a unilateral change once a standard strategy is adopted by all of the players).    

There is a rich literature of evolutionary graph theory and games played on spatial structures \citep{Nowak2006}. 
One area of this work focuses on the effect of heterogeneous network structure \citep{Santos2006} and dynamic network interactions where agents can change the connection structure of the network around them \citep{Watts2001,Szolnoki2009} including examples using the canonical coordination game \citep{Jackson2002,Goyal2005} and language evolution \citep{Selten2007}.
Much of this theory has focused on individual interactions rather than networks of populations; also, we are not aware of reports of the impact of the exact overall topology of the network structure (rather than summaries of, \textit{e.g.}, connectivity heterogenity)  on the evolution of coordination systems. There is a great deal of data on coordination game economic systems within social, geographic, and temporal networks; and these interactions could be implemented in experimental economics tests to explore network topology effects.

\subsection{Future Directions} 

A wide range of additional theoretical work to build upon these results also exists.  Here we have purposely focused on highly stable starting configurations with the population network often divided roughly in half between alternative alleles.  The full spectrum of stability from random starting configurations could be explored, as well as the establishment of alternative alleles in a smaller sector of the network. The effects of long distance dispersal, which are common among species \citep{Fraser2001} and known to destabilize underdominant polymorphims \citep{Payne2007}, could be incorporated. Furthermore, unequal migration rates (directed graphs) perhaps to incorporate current directions, homozygote fitness asymmetry, or the effects of three or more alleles could be explored \citep{Altrock2010}; however, it is anticipated that this will result in a highly complex parameter space.  For highly motivated cases, such as transforming mosquito populations in defined regions, spatially explicit models incorporating known biological parameters could be explored to refine real-world application strategies.  Finally, all natural systems exist in finite numbers.  Underdominant polymorphsims are ultimately unstable in a network of finite populations. The question then becomes how long will variation persist until it is lost and is there a bias among alternative absorbing boundaries in where the system will arrive, which influence strategies to utilize underdominance and may inform our understanding of natural systems \citep{Altrock2011}.  The effects of a network topology upon these finite populations experiencing stochastic genetic drift can also be explored.

\end{document}
